# Supplementary material for: Atomistic perspective of long lifetimes of small skyrmions at room temperature
Source: arXiv:2003.10358 ancillary file (2020-03-23)
Supplement: Supplementary file 1 [file Supplement.pdf]

# Supplemental Material for: Atomistic perspective of long lifetimes of small skyrmions at room temperature

Markus Hoffmann,* Gideon P. Müller, and Stefan Blügel
*Peter Grünberg Institut and Institute for Advanced Simulation, Forschungszentrum Jülich and JARA, 52425 Jülich Germany*
(Dated: March 23, 2020)

## SUPPLEMENTARY NOTE 1: HARMONIC TRANSITION STATE THEORY

In the main text, the harmonic transition state theory [1] (HTST) is used for the estimation of transition rates, in particular the radial collapse of a skyrmion into the ferromagnetic state. Here, we provide some details on this method.

Within the harmonic approximation to transition-state theory, the transition rate can be written

$$\Gamma^{\mathrm{HTST}}(T) = \Gamma_0(T)\, e^{-\Delta E/k_{\mathrm{B}}T} \tag{1}$$

$$= \frac{1}{2\pi} v\, \Omega_0\, \theta(T)\, \frac{V^{\mathrm{S}}}{V^{\mathrm{M}}} e^{-\Delta E/k_{\mathrm{B}}T}\,, \tag{2}$$

with

$$v = \sqrt{\sum_i{}' \frac{a_i^2}{\lambda_i^{\mathrm{S}}}}\,, \tag{3}$$

$$\Omega_0 = \sqrt{\frac{\det' H^{\mathrm{M}}}{\det' H^{\mathrm{S}}}} = \sqrt{\frac{\prod'_i \lambda_i^{\mathrm{M}}}{\prod'_i \lambda_i^{\mathrm{S}}}}\,, \tag{4}$$

$$\theta(T) = \sqrt{2\pi k_{\mathrm{B}} T}^{\left(N_0^{\mathrm{M}} - N_0^{\mathrm{S}}\right)}\,. \tag{5}$$

Note that the rate's units of $1/s$ stem from the velocity factor $v$, as all other terms' units cancel out. Here, the superscripts M and S indicate the minimum and first-order saddle point of the transition. $N_0$ are the respective number of zero modes, *i.e.* modes with zero eigenvalue, and the $V$ are the phase-space volumes of those zero modes. The $\lambda_i$ are eigenvalues of the Hessian matrix and $a_i$ are coefficients in the expansion of the velocity along the unstable mode. The primes next to determinants, products, and sums denote that only positive eigenvalues are taken into account.

Consequently, the lifetime prefactor plotted in the main text reads

$$\tau_0(T) = 1/\Gamma_0(T) = \frac{2\pi}{v\Omega_0} \sqrt{2\pi k_{\mathrm{B}} T}^{\left(N_0^{\mathrm{S}} - N_0^{\mathrm{M}}\right)} \frac{V^{\mathrm{M}}}{V^{\mathrm{S}}}\,. \tag{6}$$

We note that the calculation of zero mode volumes is found in the supplementary material of [2]. In the context of room temperature, thermal fluctuations of $\approx 300\, k_{\mathrm{B}}$ can become large compared to the energy barrier of the saddle point translation. This effectively turns the translation modes into zero modes, removing the temperature dependence in the prefactor and reducing the attempt rate prefactor. In our estimation, these two effects support the skyrmion stability at room temperature with our calculations shown in the main text representing a conservative estimation of the lifetime.

## SUPPLEMENTARY NOTE 2: LONG-RANGE EXCHANGE INTERACTION BEYOND NEXT-NEAREST NEIGHBORS

In the main text, we analyzed the dependence of the energy barrier as well as the lifetime prefactor on the competition of nearest neighbors (NN) and next-nearest neighbors (NNN) exchange interactions. Here, we extend this analysis and include also third-nearest neighbor interactions within the hexagonal monolayer. To keep the same micromagnetic value as in the main text, the values of $J_1$, $J_2$, and $J_3$ are chosen such that

$$J_1 + 3J_2 + 4J_3 = 18\mathrm{meV}\,. \tag{7}$$

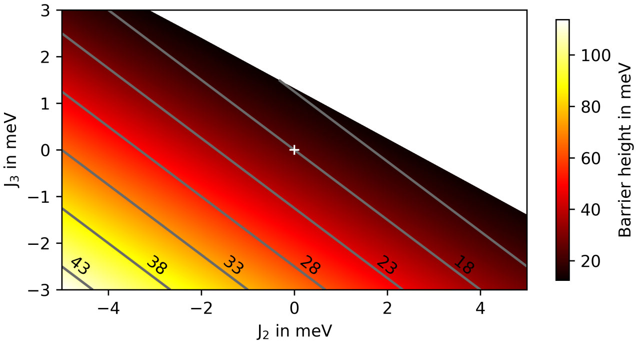


FIG. 1. Energy barrier for the collapse of a single skyrmion in dependence on the exchange interaction values. The color code represents the barrier heights obtained by GNEB calculations. As a guide for the eye, the corresponding values of $J_1$ are indicated by the gray lines and the case of $J_2 = J_3 = 0$, ie. zero frustration, is highlighted by a white cross.

Fig. 1 shows the dependence of the skyrmion collapse energy barrier on the exchange values of the first-, second-, and third-nearest neighbor pairs. It is increased significantly for frustration in both $J_2$ and $J_3$. We thus conclude that skyrmion lifetimes even beyond the range

shown in the main text can be obtained by material specific tuning of long-range interactions.

## SUPPLEMENTARY NOTE 3: DEPENDENCE OF EIGENMODES AT SADDLE POINT AND SKYRMION MINIMUM ON VARIATION OF INTERACTION PARAMETERS

In the main text, we presented the lifetime prefactor of the skyrmion collapse in dependence on the atomistic parameters, more precisely the strength of NNN interactions compared to NN ones both in exchange as well as in DMI. A quite complex behavior could be seen which we addressed to the complex interplay of the parameter dependence of eigen modes in the skyrmion as well as in the saddle point which enter the skyrmion lifetime as given in (5). Figure 2 shows this dependence for the four modes with lowest excitation energy [3], *i.e.* the breathing, translation, core shift, and chirality change mode in case of the saddle point configuration and the breathing, chirality change, core shift, and elliptical instability at the minimum. It can be clearly seen that their dependencies on the choice of the atomistic parameters are significantly different, resulting in the prefactor as shown in the main text.

* m.hoffmann@fz-juelich.de

[1] P. F. Bessarab, V. M. Uzdin, and H. Jónsson, Phys. Rev. B **85**, 184409 (2012).
[2] P. F. Bessarab, G. P. Müller, I. S. Lobanov, F. N. Rybakov, N. S. Kiselev, H. Jónsson, V. M. Uzdin, S. Blügel, L. Bergqvist, and A. Delin, Sci. Rep. **8**, 3433 (2018).
[3] Please notice: the modes are ordered with respect to their eigenvalues for the case $J_2 = |\mathbf{D}_2| = 0$. Due to their different dependence on those parameters, crossing can occur, changing the order of the modes.

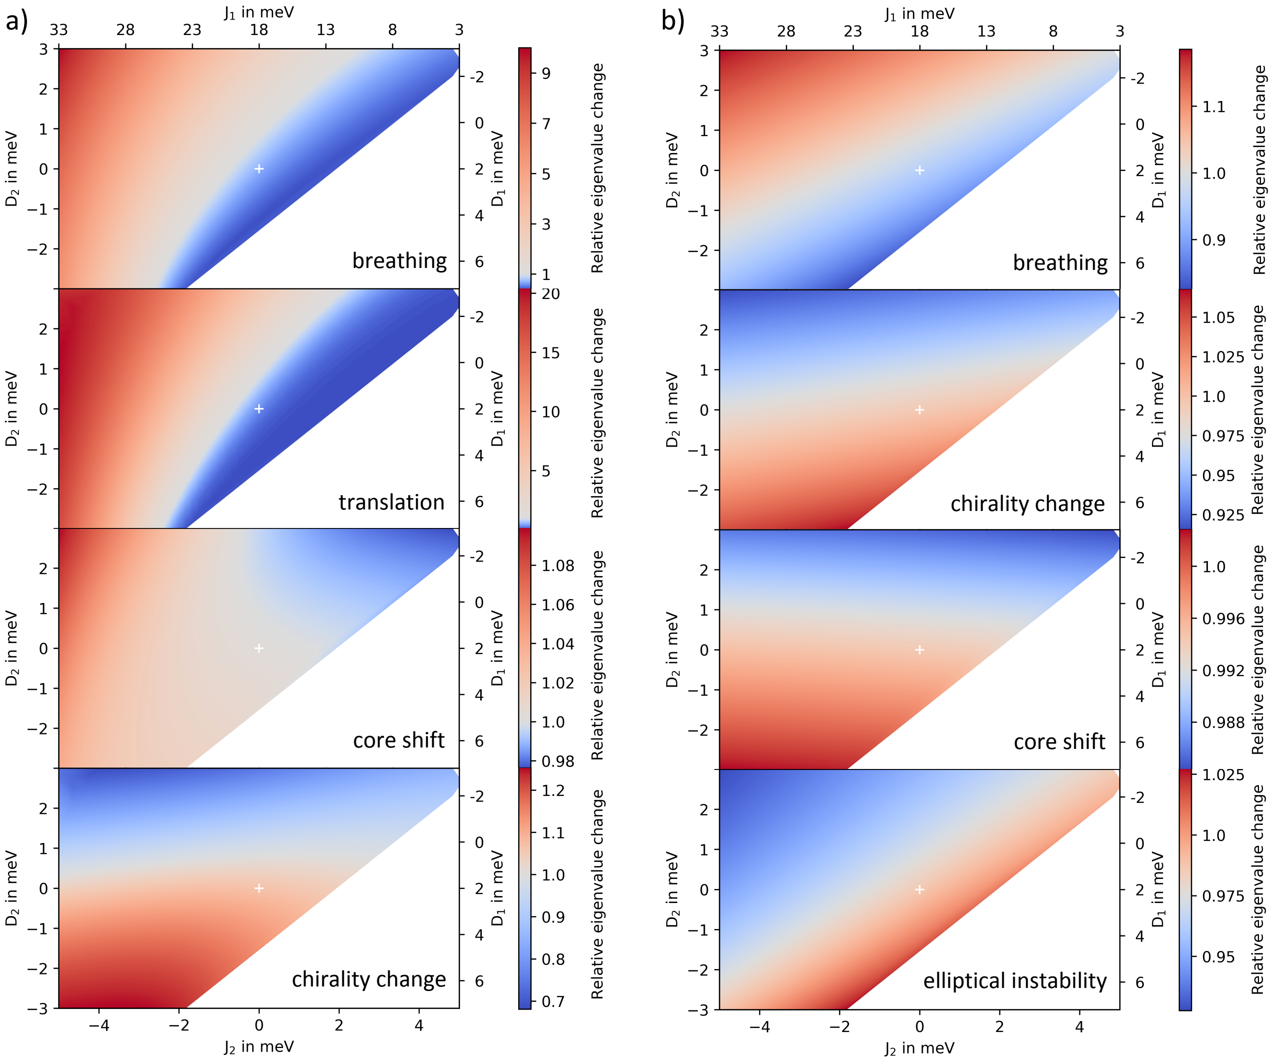


FIG. 2. The relative change of eigenvalues of distinct a) saddle point and b) skyrmion modes at the local minimum are shown in dependence on the values of exchange interaction and DMI. As a reference, the case $J_2 = |\mathbf{D}_2| = 0$ was chosen. Please notice the different color scales.
